# Supplementary material for: Impact of temporal correlations, coherence, and postselection on two-photon interference
Source: arXiv:2312.01503 ancillary file (2024-02-18)
Supplement: Supplementary file 1 [file supplemental.pdf]

# Supplemental Material: Impact of temporal correlations, coherence, and postselection on two-photon interference

Fernando Redivo Cardoso,[1,2] Jaewon Lee,[2] Riccardo Checchinato,[2] Jan-Heinrich Littmann,[2] Marco De Gregorio,[3] Sven Höfling,[3] Christian Schneider,[4] Celso J. Villas-Boas,[1] and Ana Predojević[2,*]

[1]*Departamento de Física, Universidade Federal de São Carlos, 13565-905 São Carlos, São Paulo, Brazil*
[2]*Department of Physics, Stockholm University, 10691 Stockholm, Sweden*
[3]*Technische Physik, Physikalisches Institut and Würzburg-Dresden Cluster of Excellence ct.qmat, Universität Würzburg, Am Hubland, D-97074 Würzburg, Germany*
[4]*Institut of Physics, University of Oldenburg, D-26129 Oldenburg, Germany*

Two-photon interference is an indispensable resource in quantum photonics, but it is not straightforward to achieve. The cascaded generation of photon pairs contains intrinsic temporal correlations that negatively affect the ability of such sources to perform two-photon interference, thus hindering applications. We report on how such correlation interplays with decoherence and temporal postselection, and under which conditions temporal postselection could improve two-photon interference visibility. Our study identifies crucial parameters and points the way to a source with optimal performance.

## I. THE QUANTUM DOT PHOTON PAIR SOURCE

To perform the measurements, we used a quantum dot embedded in a micropillar cavity. The cavity was designed to consist of 5 top and 18 bottom pairs of $\lambda/4$ thick AlAs/GaAs distributed Bragg reflectors. The diameter of the micropillar was 2.74 $\mu$m. The sample was kept in a closed-cycle cryostat at 5.273(23) K. The quantum dot emission was collected using a 0.7 NA aspherical lens. We eliminated the excess laser scattering using a polarizer and a notch filter with a bandwidth of 0.65 nm. The single-photon nature of the emission was confirmed by measuring the autocorrelation function, as shown in Fig. 1. The results of the biexciton and exciton lifetime measurement are presented in Fig. 2a, along with the respective fits.

## II. QUANTUM DOT LEVEL STRUCTURE AND SYSTEM DYNAMICS

In the interaction picture, the Hamiltonian for the three-level system can be expressed as follows

$$H_I = \Delta_x \sigma_{xx} + \frac{\Omega(t)}{2}\left(\sigma_{xg} + \sigma_{bx} + \mathrm{h.c.}\right) \tag{1}$$

with $\sigma_{ij} = |i\rangle\langle j|$. The two-photon resonance is detuned from the single-photon resonance (ground state, $|g\rangle$, to exciton, $|x\rangle$) by $\Delta_x$, which is equal to $2\pi \times 434$ GHz for the system we studied. We assume the laser excitation pulse to have a Gaussian profile with the following form

$$\Omega(t) = \Omega_0 \mathrm{e}^{-2\log(2)\left(\frac{t-t_0}{\sigma}\right)^2}, \tag{2}$$

where $\Omega_0$ is the Rabi frequency. The intensity of the pulse peaks at $t = t_0$ and the pulse width is $\sigma$. Upon the quantum dot excitation the biexciton photon, $\omega_1$, and exciton photon, $\omega_2$, are emitted. The biexciton and exciton decay rates are $\Gamma_b$ and $\Gamma_x$, respectively. The frequencies of the emitted photons are related as $\omega_2 > \omega_L > \omega_1$ (see Figure 1a in the main text). The biexciton and exciton lifetimes are $\tau_b$ and $\tau_x$, respectively.

The system dynamics can be obtained by solving the master equation for the density operator $\rho$,

$$\dot{\rho} = -\mathrm{i}[H_I, \rho] + \sum_k \mathcal{L}_k \rho. \tag{3}$$

Here, the $\mathcal{L}_k$ ($k = 1, 2$) are the Lindblad terms that account for spontaneous decay

$$\mathcal{L}_1\rho = \frac{\Gamma_b}{2}\left[2\sigma_{xb}\rho\sigma_{xb}^\dagger - \sigma_{xb}^\dagger\sigma_{xb}\rho - \rho\sigma_{xb}^\dagger\sigma_{xb}\right], \tag{4}$$

$$\mathcal{L}_2\rho = \frac{\Gamma_x}{2}\left[2\sigma_{gx}\rho\sigma_{gx}^\dagger - \sigma_{gx}^\dagger\sigma_{gx}\rho - \rho\sigma_{gx}^\dagger\sigma_{gx}\right], \tag{5}$$

and dephasing $\mathcal{L}_k$ ($k = 3, 4$)

$$\mathcal{L}_3\rho = \frac{\Gamma_{\mathrm{db}}}{2}\left[2\sigma_{\mathrm{db}}\rho\sigma_{\mathrm{db}}^\dagger - \sigma_{\mathrm{db}}^\dagger\sigma_{\mathrm{db}}\rho - \rho\sigma_{\mathrm{db}}^\dagger\sigma_{\mathrm{db}}\right], \tag{6}$$

$$\mathcal{L}_4\rho = \frac{\Gamma_{\mathrm{db}}}{2}\left[2\sigma_{\mathrm{dx}}\rho\sigma_{\mathrm{dx}}^\dagger - \sigma_{\mathrm{dx}}^\dagger\sigma_{\mathrm{dx}}\rho - \rho\sigma_{\mathrm{dx}}^\dagger\sigma_{\mathrm{dx}}\right], \tag{7}$$

with $\sigma_{\mathrm{db}} = \sigma_{bb} - \sigma_{xx}$ and $\sigma_{\mathrm{dx}} = \sigma_{xx} - \sigma_{gg}$. The factors $\Gamma_{\mathrm{db,dx}} = (1/\tau_{\mathrm{db,dx}})$ are the dephasing rates of biexciton and exciton, respectively. For the simulations, the population of the biexciton state, defined by

$$P_b = \Gamma_b \int_0^\infty \langle\sigma_{bb}(t)\rangle\,\mathrm{d}t, \tag{8}$$

was adjusted via $\Omega_0$ to the value of $P_b = 0.5$. Figure 2b illustrates the biexciton and exciton population as a function of time. Figure 2c shows the 2D histogram of the biexciton and exciton emission times. The triangular shape of the 2D histogram indicates correlation that originates in the temporal ordering of the photon emission, mathematically described by two-photon wave function $\psi(t_b, t_x)$, given in the main text.

* ana.predojevic@fysik.su.se

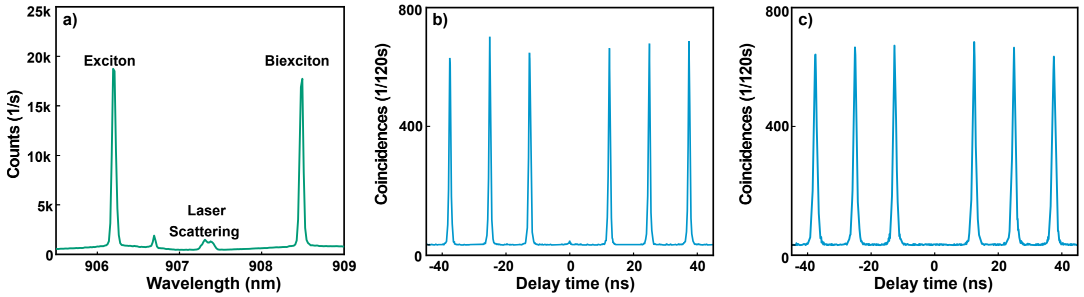


FIG. 1. a) Quantum dot emission spectrum, measured under two-photon resonant excitation. b) The results of auto-correlation measurements for b) biexciton and c) exciton. The measurements yield $g_b^{(2)}(0)$=0.0144(19) and $g_x^{(2)}(0)$=0.0074(11) for biexciton and exciton, respectively.

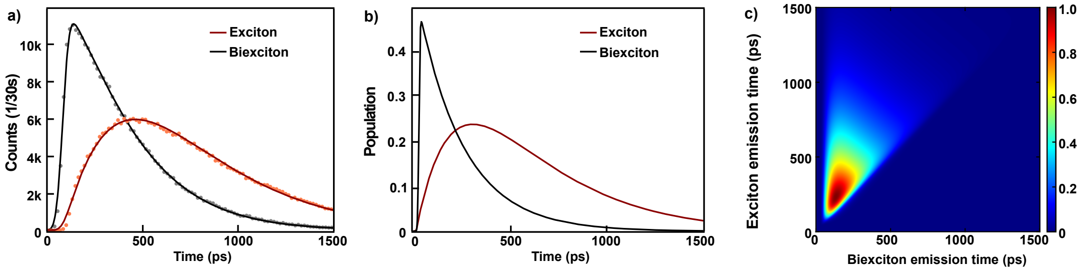


FIG. 2. a) Results of the biexciton and exciton lifetime measurements. We employed a 35 ps resolution single photon detector. From the data fit we deduct the lifetimes of $\tau_b = 237.16(59)$ ps and $\tau_x = 367.61(99)$ ps for the biexciton and exciton, respectively. b) Simulated quantum dot populations for biexciton ($|b\rangle$) and exciton ($|x\rangle$) as a function of time. The lifetimes were considered to be $\tau_b$ and $\tau_x$, determined experimentally. c) 2D histogram of the emission times of the biexciton and exciton. The triangular shape reflects the time ordering of the emitted photons. The correlation intensity is normalized to unity.

## III. SENSOR METHOD

As introduced in the main text the sensor method supplements the three-level system with 2 two-level systems, one per emission frequency. These two-level systems act as sensors and, as given in the main text, are described by the following Hamiltonian:

$$H_s = \sum_{j=1}^{2} \left\{ \omega_j \xi_j^\dagger \xi_j + g \left[ (\sigma_{xb} + \sigma_{gx}) \xi_j^\dagger + \text{h.c.} \right] \right\}. \quad (9)$$

Upon performing a unitary transformation, the complete Hamiltonian of the system can be written as

$$\begin{aligned} H' = \Delta_x \sigma_{xx} + \omega_1 \xi_1^\dagger \xi_1 + \omega_2 \xi_2^\dagger \xi_2 \\ + \frac{\Omega(t)}{2} (\sigma_{gx} + \sigma_{xb} + \text{h.c.}) \\ + g \sum_{j=1}^{2} \left[ (\sigma_{xb} + \sigma_{gx}) \xi_j^\dagger \mathrm{e}^{-\mathrm{i}\omega_L t} + \text{h.c.} \right] \end{aligned} \quad (10)$$

where the terms that oscillate with double the laser frequency have been eliminated. To make the Hamiltonian time independent, we perform two unitary transformations involving sensor operators. The first transformation is $U_2 = \mathrm{e}^{-\mathrm{i}H_2 t}$, with $H_2$ being the free part of the sensor Hamiltonian

$$H_2 = \omega_1 \xi_1^\dagger \xi_1 + \omega_2 \xi_2^\dagger \xi_2. \quad (11)$$

By defining the sensor detunings $\Delta_i = \omega_i - \omega_L$ $(i = 1, 2)$, the Hamiltonian is transformed to

$$\begin{aligned} H'' = \Delta_x |x\rangle\langle x| + \frac{\Omega(t)}{2} (|g\rangle\langle x| + |x\rangle\langle b| + \text{h.c.}) \\ + \epsilon \sum_{i=1}^{2} \left[ (\sigma_{xb} + \sigma_{gx}) \mathrm{e}^{\mathrm{i}\Delta_i t} \xi_i^\dagger + \text{h.c.} \right]. \end{aligned} \quad (12)$$

In the second transformation, the time dependence from the sensor coupling terms is removed using the following unitary operation $U_3 = \mathrm{e}^{-\mathrm{i}H_3 t}$, with

$$H_3 = \alpha_1 \xi_1^\dagger \xi_1 + \alpha_2 \xi_2^\dagger \xi_2, \quad (13)$$

where $\alpha$ coefficients are to be determined. The transformation acts on $H''$ in the following way

$$\begin{aligned} H_I = -\alpha_1 \xi_1^\dagger \xi_1 - \alpha_2 \xi_2^\dagger \xi_2 + \Delta_x |x\rangle\langle x| \\ + \frac{\Omega(t)}{2} (|g\rangle\langle x| + |x\rangle\langle b| + \text{h.c.}) \\ + g \sum_{j=1}^{2} \left[ (\sigma_{xb} + \sigma_{gx}) \mathrm{e}^{\mathrm{i}(\Delta_j + \alpha_j)t} \xi_j^\dagger + \text{h.c.} \right], \end{aligned} \quad (14)$$

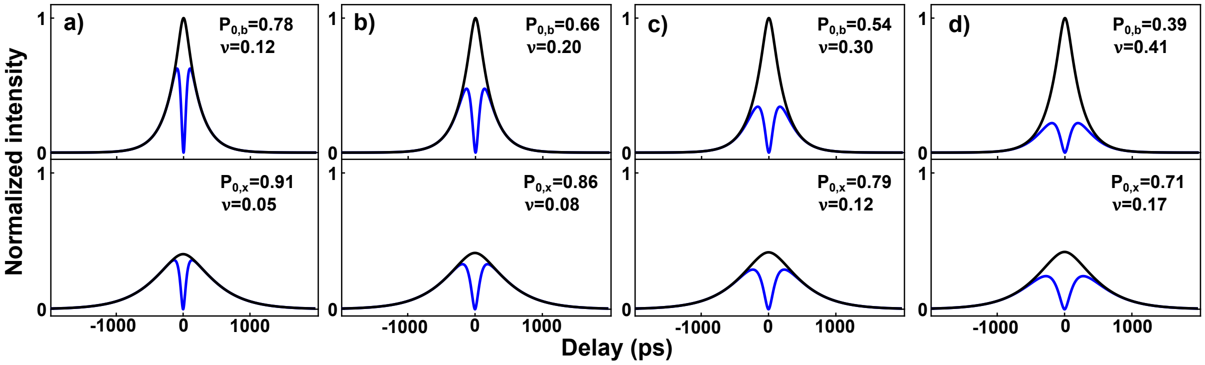


FIG. 3. Simulated values of $G^{(2)}_{HOM}(\tau)$ (in blue) obtained using sensor method and accounting for dephasing of the quantum dot levels. The coherence time of both biexciton and exciton were chosen to be a) 100 ps, b) 200 ps, c) 300 ps d) 400 ps. The top image shows the $G^{(2)}_{HOM}(\tau)$ of the biexciton while the bottom one shows the $G^{(2)}_{HOM}(\tau)$ of the exciton. for better comparison on each image is shown the mode intensity (in black). While the selected coherence times are equal for the biexciton and, exciton the achieved values of the $P(\tau)$ and visibility ($\nu$) (shown in each plot) are quite different.

resulting in a Hamiltonian that is time independent under the following conditions

$$\begin{cases} \Delta_1 + \alpha_1 = 0 \Rightarrow -\alpha_1 = \Delta_1 \\ \Delta_2 + \alpha_2 = 0 \Rightarrow -\alpha_2 = \Delta_2. \end{cases} \tag{15}$$

We employ this result to rewrite the time independent Hamiltonian as

$$\begin{aligned} H_I = \Delta_1 \xi_1^\dagger \xi_1 + \Delta_2 \xi_2^\dagger \xi_2 + \Delta_x |x\rangle\langle x| \\ + \frac{\Omega(t)}{2} \left( |g\rangle\langle x| + |x\rangle\langle b| + \text{h.c.} \right) \\ + g \sum_{j=1}^{2} \left[ \left( \sigma_{xb} + \sigma_{gx} \right) \xi_j^\dagger + \text{h.c.} \right]. \end{aligned} \tag{16}$$

This adjustment in eq. (16) enables the sensors to be resonant to the respective optical transitions of the three level system. To this end, the sensor detunings $\Delta_1$ and $\Delta_2$ are chosen to be

$$\begin{aligned} \omega_1 &= \omega_b - \omega_x \\ \omega_1 - \omega_L &= (\omega_b - \omega_x) - \omega_L + \omega_L - \omega_L \\ \Delta_1 &= -\Delta_x, \end{aligned} \tag{17}$$

for sensor 1, and

$$\begin{aligned} \omega_2 &= \omega_x - \omega_g \\ \omega_2 - \omega_L &= \omega_x - \omega_L \\ \Delta_2 &= \Delta_x. \end{aligned} \tag{18}$$

for sensor 2. Finally, we consider each of the sensors to have a linewidth. These manifest as two additional Lindblad terms that we add to the master equation,

$$\mathcal{L}_j \rho = \frac{\kappa_j}{2} \left( 2\xi_j \rho \xi_j^\dagger - \xi_j^\dagger \xi_j \rho - \rho \xi_j^\dagger \xi_j \right), \tag{19}$$

with $j = 1, 2$.

In our study, we use the sensor method where two quantized modes act as weakly coupled sensors to model the behavior of a detector. A notable advantage of this framework is its ability to compute $N$-photon correlations for arbitrary time delays and frequencies, making it suitable for application to any open quantum system. Since the emissions ultimately occur in free space, we assume that the linewidth $\kappa_j$ associated with each of the sensors is broadband ($\kappa \gg 1$). The coupling strengths ($g$) associated with the sensors are made small, satisfying $\epsilon_j \ll \sqrt{\kappa_j \gamma_j / 2}$, to prevent the introduction of feedback into the main system. The sensor method has been previously developed and used to study photon-photon correlations in various physical systems [1, 2]. Moreover, no additional assumptions are imposed on the system, and the correlation functions obtained with the sensor operators correspond to the correlations in emission [3]. We employ and demonstrate the applicability of the sensor method to investigate time-resolved correlations, as well as to model the emission and two-photon interference of photons emitted as a part of the biexciton-exciton cascade.

## IV. TWO-PHOTON INTERFERENCE

The Hong-Ou-Mandel (HOM) or two-photon interference manifests when two photons impinge on distinct ports of a beamsplitter. The photons will interfere, depending on their degree of indistinguishability. We investigated the two-photon interference of the consecutively emitted biexciton (exciton) photons while considering the inherent correlations present in biexciton-exciton cascade.

Our analysis considers as parameters the lifetimes of biexciton and exciton as well as the dephasing resulting from the drifting of the internal levels, all of which can exert an impact on the interference visibility of the generated photons. The two-photon interference properties are obtained, as explained in the main text, via the correlations of the auxiliary two-level

TABLE I. Values of the visibility, $\nu$, for biexciton two-photon interference for the quantum dot we used in our measurements. The exciton coherence times are given in the row most to the left, while the values of the biexciton coherence time are given in the top column. All coherence times are in ps.

| | 50 | 100 | 150 | 200 | 250 | 300 | 350 | 400 |
|---|---|---|---|---|---|---|---|---|
| 50 | 0.087 | 0.112 | 0.129 | 0.143 | 0.153 | 0.162 | 0.169 | 0.175 |
| 100 | 0.092 | 0.124 | 0.151 | 0.175 | 0.196 | 0.215 | 0.233 | 0.249 |
| 150 | 0.093 | 0.129 | 0.162 | 0.192 | 0.221 | 0.249 | 0.276 | 0.302 |
| 200 | 0.094 | 0.132 | 0.168 | 0.203 | 0.237 | 0.272 | 0.307 | 0.343 |
| 250 | 0.095 | 0.134 | 0.172 | 0.210 | 0.249 | 0.289 | 0.331 | 0.375 |
| 300 | 0.095 | 0.136 | 0.175 | 0.215 | 0.257 | 0.302 | 0.350 | 0.401 |
| 350 | 0.095 | 0.136 | 0.177 | 0.219 | 0.264 | 0.312 | 0.365 | 0.422 |
| 400 | 0.095 | 0.137 | 0.179 | 0.222 | 0.269 | 0.321 | 0.377 | 0.440 |
| 450 | 0.096 | 0.138 | 0.180 | 0.225 | 0.274 | 0.328 | 0.388 | 0.456 |
| 500 | 0.096 | 0.138 | 0.181 | 0.227 | 0.277 | 0.334 | 0.397 | 0.469 |
| 550 | 0.096 | 0.139 | 0.182 | 0.229 | 0.281 | 0.338 | 0.404 | 0.481 |
| 600 | 0.096 | 0.139 | 0.183 | 0.230 | 0.283 | 0.343 | 0.411 | 0.491 |
| 650 | 0.096 | 0.139 | 0.184 | 0.232 | 0.285 | 0.346 | 0.417 | 0.500 |
| 700 | 0.096 | 0.139 | 0.184 | 0.233 | 0.287 | 0.350 | 0.422 | 0.508 |
| 750 | 0.096 | 0.140 | 0.185 | 0.234 | 0.289 | 0.353 | 0.427 | 0.515 |

TABLE II. Values of visibility, $\nu$, for exciton interference, for the quantum dot we used in our measurements. The exciton coherence times are given in the column most to the left, while the values of the biexciton coherence time are given in the top row. All coherence times are in ps.

| | 50 | 100 | 150 | 200 | 250 | 300 | 350 | 400 |
|---|---|---|---|---|---|---|---|---|
| 50 | 0.033 | 0.035 | 0.035 | 0.036 | 0.036 | 0.036 | 0.036 | 0.036 |
| 100 | 0.042 | 0.047 | 0.049 | 0.050 | 0.051 | 0.052 | 0.052 | 0.052 |
| 150 | 0.049 | 0.058 | 0.062 | 0.064 | 0.066 | 0.067 | 0.068 | 0.068 |
| 200 | 0.054 | 0.067 | 0.073 | 0.077 | 0.080 | 0.082 | 0.084 | 0.085 |
| 250 | 0.058 | 0.075 | 0.085 | 0.091 | 0.095 | 0.099 | 0.101 | 0.103 |
| 300 | 0.062 | 0.082 | 0.095 | 0.104 | 0.111 | 0.116 | 0.120 | 0.123 |
| 350 | 0.064 | 0.089 | 0.106 | 0.118 | 0.127 | 0.135 | 0.141 | 0.146 |
| 400 | 0.067 | 0.095 | 0.116 | 0.132 | 0.145 | 0.155 | 0.164 | 0.171 |
| 450 | 0.069 | 0.101 | 0.126 | 0.146 | 0.163 | 0.177 | 0.189 | 0.199 |
| 500 | 0.070 | 0.106 | 0.136 | 0.161 | 0.182 | 0.201 | 0.217 | 0.232 |
| 550 | 0.072 | 0.111 | 0.145 | 0.176 | 0.203 | 0.227 | 0.249 | 0.269 |
| 600 | 0.073 | 0.116 | 0.155 | 0.191 | 0.225 | 0.256 | 0.286 | 0.313 |
| 650 | 0.074 | 0.120 | 0.164 | 0.207 | 0.248 | 0.288 | 0.327 | 0.366 |
| 700 | 0.076 | 0.124 | 0.173 | 0.223 | 0.273 | 0.324 | 0.376 | 0.430 |
| 750 | 0.077 | 0.128 | 0.182 | 0.239 | 0.300 | 0.364 | 0.434 | 0.508 |

systems, i.e. sensors.

In figure 3 are shown several examples of $G^{(2)}_{HOM}(\tau)$ calculated for various values of the coherence length of the biexciton and the exciton. The figures clearly demonstrate that even for the same values of the coherence length the biexciton and exciton will not exhibit the same $P_0$ and $\nu$. Namely the potential to perform two-photon interference is always stronger with biexciton photon. On the other hand, and as shown in the Fig. 1 of the main text the cascade correlation alone induces equal reduction of the interference contrast.

In the tables I and II we give the numerical values of the visibility for biexicton and exciton, respectively. These values have been calculated for the quantum dot emitter that we em-

TABLE III. Values of visibility, $\nu$, for biexciton two-photon interference for the ratio of 2 between the lifetimes of the exciton and biexciton (400 ps and 200 ps, respectively). The first column on the left contains exciton coherence times, while the top row contains biexciton coherence times. All values are given in ps.

| | 50 | 100 | 150 | 200 | 250 | 300 | 350 | 400 |
|---|---|---|---|---|---|---|---|---|
| 50 | 0.090 | 0.115 | 0.134 | 0.147 | 0.158 | 0.167 | 0.175 | 0.181 |
| 100 | 0.094 | 0.128 | 0.156 | 0.181 | 0.204 | 0.224 | 0.242 | 0.258 |
| 150 | 0.096 | 0.134 | 0.167 | 0.199 | 0.230 | 0.260 | 0.289 | 0.315 |
| 200 | 0.097 | 0.137 | 0.174 | 0.211 | 0.247 | 0.284 | 0.322 | 0.358 |
| 250 | 0.097 | 0.139 | 0.178 | 0.218 | 0.260 | 0.303 | 0.348 | 0.392 |
| 300 | 0.098 | 0.140 | 0.181 | 0.224 | 0.269 | 0.317 | 0.369 | 0.420 |
| 350 | 0.098 | 0.141 | 0.184 | 0.228 | 0.276 | 0.328 | 0.385 | 0.443 |
| 400 | 0.098 | 0.142 | 0.185 | 0.231 | 0.282 | 0.337 | 0.399 | 0.463 |
| 450 | 0.098 | 0.142 | 0.187 | 0.234 | 0.286 | 0.345 | 0.411 | 0.480 |
| 500 | 0.099 | 0.143 | 0.188 | 0.236 | 0.290 | 0.351 | 0.420 | 0.494 |
| 550 | 0.099 | 0.143 | 0.189 | 0.238 | 0.294 | 0.356 | 0.429 | 0.507 |
| 600 | 0.099 | 0.144 | 0.190 | 0.240 | 0.296 | 0.361 | 0.436 | 0.518 |
| 650 | 0.099 | 0.144 | 0.190 | 0.241 | 0.299 | 0.365 | 0.443 | 0.528 |
| 700 | 0.099 | 0.144 | 0.191 | 0.242 | 0.301 | 0.369 | 0.449 | 0.536 |
| 750 | 0.099 | 0.144 | 0.191 | 0.244 | 0.303 | 0.372 | 0.454 | 0.544 |
| 800 | 0.099 | 0.144 | 0.192 | 0.244 | 0.304 | 0.374 | 0.458 | 0.551 |

TABLE IV. Values of visibility, $\nu$, for exciton two-photon interference for the ratio of 2 between the lifetimes of the exciton and biexciton (400 ps and 200 ps, respectively). The first column on the left contains exciton coherence times, while the top row contains biexciton coherence times. All values are given in ps.

| | 50 | 100 | 150 | 200 | 250 | 300 | 350 | 400 |
|---|---|---|---|---|---|---|---|---|
| 50 | 0.032 | 0.034 | 0.034 | 0.035 | 0.035 | 0.035 | 0.035 | 0.035 |
| 100 | 0.041 | 0.046 | 0.048 | 0.049 | 0.050 | 0.050 | 0.051 | 0.051 |
| 150 | 0.048 | 0.056 | 0.060 | 0.062 | 0.064 | 0.065 | 0.066 | 0.066 |
| 200 | 0.053 | 0.065 | 0.071 | 0.075 | 0.078 | 0.080 | 0.081 | 0.083 |
| 250 | 0.057 | 0.073 | 0.082 | 0.088 | 0.093 | 0.096 | 0.098 | 0.100 |
| 300 | 0.060 | 0.080 | 0.093 | 0.101 | 0.108 | 0.112 | 0.116 | 0.119 |
| 350 | 0.063 | 0.086 | 0.103 | 0.114 | 0.123 | 0.130 | 0.136 | 0.140 |
| 400 | 0.065 | 0.092 | 0.112 | 0.128 | 0.140 | 0.150 | 0.158 | 0.164 |
| 450 | 0.067 | 0.098 | 0.122 | 0.141 | 0.157 | 0.170 | 0.182 | 0.191 |
| 500 | 0.068 | 0.103 | 0.131 | 0.155 | 0.175 | 0.193 | 0.208 | 0.221 |
| 550 | 0.070 | 0.108 | 0.141 | 0.169 | 0.195 | 0.218 | 0.238 | 0.256 |
| 600 | 0.071 | 0.112 | 0.150 | 0.184 | 0.215 | 0.245 | 0.272 | 0.296 |
| 650 | 0.072 | 0.117 | 0.158 | 0.198 | 0.237 | 0.275 | 0.311 | 0.344 |
| 700 | 0.073 | 0.121 | 0.167 | 0.214 | 0.261 | 0.308 | 0.356 | 0.401 |
| 750 | 0.074 | 0.124 | 0.175 | 0.229 | 0.285 | 0.345 | 0.408 | 0.469 |

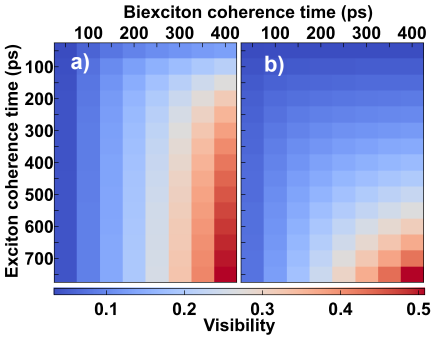


FIG. 4. The panels a) and b) show the visibility of the biexciton and exciton photon respectively for various values of the biexciton and exciton photon coherence time. The numerical values are given in tables III and IV.

ployed in the experiments. These values of the visibility are also graphically presented in the the Figure 2e and 2f of the main text.

In addition to this we also have calculated the values of the visibility for an emitter that has the ratio of 2:1 between the exciton and the biexciton lifetime (400 ps and 200 ps, respectively). These values are shown in the the tables III and IV, while the plot is shown in the Figure 4.

[1] M. Peiris, B. Petrak, K. Konthasinghe, Y. Yu, Z. C. Niu, and A. Muller, Phys. Rev. B **91**, 195125 (2015).

[2] E. Darsheshdar, M. Hugbart, R. Bachelard, and C. J. Villas-Boas, Phys. Rev. A **103**, 053702 (2021).

[3] E. del Valle, A. Gonzalez-Tudela, F. P. Laussy, C Tejedor, M. J. Hartmann, Phys. Rev. Lett. **109**, 183601 (2012).

[4] H. Carmichael Statistical Methods in Quantum Optics 1: master equations and Fokker-Planck equations, Springer Science and Business Media (1999).
